# Supplementary material for: Deterministic delivery of remote entanglement on a quantum network
Source: arXiv:1712.07567 ancillary file (2018-01-15)
Supplement: Supplementary file 1 [file SupplementaryInformation.pdf]

Supplementary Information for

# Deterministic delivery of remote entanglement on a quantum network


Peter C. Humphreys,[1,*] Norbert Kalb,[1,*] Jaco P. J. Morits,[1] Raymond N. Schouten,[1] Raymond F. L. Vermeulen,[1] Daniel J. Twitchen,[2] Matthew Markham,[2] and Ronald Hanson[1]

[1]*QuTech & Kavli Institute of Nanoscience, Delft University of Technology, PO Box 5046, 2600 GA Delft, The Netherlands*

[2]*Element Six Innovation, Fermi Avenue, Didcot, Oxfordshire OX11 0QE, U.K.*


## I. DERIVATION OF DETERMINISTICALLY DELIVERED ENTANGLED STATE FIDELITY AS A FUNCTION OF QUANTUM LINK EFFICIENCY

We assume an entanglement generation rate $r_{\mathrm{ent}}$ and an entangled state decoherence rate $r_{\mathrm{dec}}$. If the rate at which entanglement attempts occur is much faster than $r_{\mathrm{ent}}$ (i.e there is a low probability of success), we can approximate entanglement generation as a continuous process. In this case, the probability density for successfully generating entanglement at a time $t$ after beginning our attempts is given by $p_{\mathrm{ent}}(t) = r_{\mathrm{ent}} e^{-r_{\mathrm{ent}} t}$. The corresponding cumulative probability of success is $p_{\mathrm{succ}}(t) = 1 - e^{-r_{\mathrm{ent}} t}$.

Once we succeed at creating entanglement, the state will decohere until the time at which we deliver it. For single-qubit depolarising noise at each site, the fidelity of the resulting state after storage for a time $t$ is given by

$$F(t) = \frac{1}{4} + \frac{3}{4} e^{-r_{\mathrm{dec}} t}. \tag{1}$$

If we deliver our entangled state at time $t_{\mathrm{ent}} = \beta / r_{\mathrm{dec}}$ (where $\beta$ is simply used to parameterise the time in terms of the decoherence rate), the average fidelity of the delivered state (given a success occurred) is therefore

$$\begin{aligned} F_{\mathrm{succ}} &= \frac{1}{p_{\mathrm{succ}}(t_{\mathrm{ent}})} \int_0^{t_{\mathrm{ent}}} p_{\mathrm{ent}}(t) F(t_{\mathrm{ent}} - t) \mathrm{d}t \\ &= \frac{1}{p_{\mathrm{succ}}(t_{\mathrm{ent}})} \int_0^{t_{\mathrm{ent}}} r_{\mathrm{ent}} e^{-r_{\mathrm{ent}} t} \left(\frac{1}{4} + \frac{3}{4} e^{-r_{\mathrm{dec}}(t_{\mathrm{ent}} - t)}\right) \mathrm{d}t. \\ &= \frac{3 e^{-\beta} \eta_{\mathrm{link}} + (1 - 4\eta_{\mathrm{link}}) e^{-\eta_{\mathrm{link}} \beta} + \eta_{\mathrm{link}} - 1}{4(\eta_{\mathrm{link}} - 1) p_{\mathrm{succ}}(t_{\mathrm{ent}})} \end{aligned} \tag{2}$$

We note that $p_{\mathrm{succ}}(t_{\mathrm{ent}}) = 1 - e^{-\beta \eta_{\mathrm{link}}}$, and therefore $\beta = -\ln(1 - p_{\mathrm{succ}}(t_{\mathrm{ent}}))/\eta_{\mathrm{link}}$. Using this, along with the shorthand $p_{\mathrm{succ}} = p_{\mathrm{succ}}(t_{\mathrm{ent}})$, we find that

$$F_{\mathrm{succ}} = \frac{3\eta_{\mathrm{link}} + p_{\mathrm{succ}} - 3\eta_{\mathrm{link}}(1 - p_{\mathrm{succ}})^{1/\eta_{\mathrm{link}}} - 4\eta_{\mathrm{link}} p_{\mathrm{succ}}}{4 p_{\mathrm{succ}}(1 - \eta_{\mathrm{link}})}. \tag{3}$$

[*] These authors contributed equally to this work.

As discussed in the main text, we can choose to draw a black box around this process, delivering an unentangled state (state fidelity $F_{\text{unent}} \leq \frac{1}{2}$) for cycles in which no attempt at entanglement generation succeeds such that a state is always delivered. Reproducing Eq. 1 of the main text, this means that the states output from this black-box will have a fidelity with a Bell state of

$$F_{\text{det}} = p_{\text{succ}} F_{\text{succ}} + (1 - p_{\text{succ}}) F_{\text{unent}}, \tag{4}$$

where $F_{\text{succ}}$ is as given above. The maximum achievable fidelity when outputting a fully mixed state ($F_{\text{unent}} = \frac{1}{4}$) upon failure is found by optimising $F_{\text{succ}}$ for a given quantum link efficiency $\eta_{\text{link}}$:

$$F_{\text{det}}^{\text{max}} = \frac{1}{4} \left( 1 + 3 (\eta_{\text{link}})^{\frac{1}{1-\eta_{\text{link}}}} \right). \tag{5}$$

Note that the full state of a quantum system can only be determined experimentally using an ensemble of identical states. This means that, in the absence of information about which deterministic entanglement delivery cycles have a heralded success, the only accurate description of the output of such a black-box system is that a statistical mixture is deterministically output at each cycle.

## II. EXPERIMENTAL METHODS FOR DETERMINISTIC ENTANGLEMENT DELIVERY

### A. Experiment design

We use chemical-vapour-deposition homoepitaxially grown diamonds of type IIa with a natural abundance of carbon isotopes. Both diamonds have been cut along the ⟨111⟩ crystal axis and were grown by Element Six. They are situated in home-built confocal microscope set-ups within closed-cycle cryostats (4 K, Montana Instruments) separated by two meters. We use fast microwave switches to shield both NV centres from microwave amplifier noise and therefore increase the coherence times dramatically (Node A uses Qorvo TGS2355-SM and Node B uses Analog Devices HMC544). All other parts of the set-up and sample details have been described in the Supplementary Information of Refs. [1, 2].

One cycle of the deterministic entanglement protocol consists of optical phase stabilisation (described in detail in Sec. V), charge-resonance checks to ensure that both NVs are in the appropriate charge state and on-resonance [3], heralded single-photon entanglement generation, and finally dynamical decoupling to protect the state of the NVs from their environment until the delivery time. The experimental sequences used in each step of this protocol (and also the single-photon entanglement generation experiment) are detailed in Supp. Fig. 1.

After delivery, the state of each NV is measured in a chosen basis. We use spin-selective optical read-out of the NV electron spin in a single shot via the optical $E_x$ transition on both nodes [3]. We measure single-shot read-out fidelities of 0.959(3) (0.950(3)) for the bright $|m_s = 0\rangle \equiv |\uparrow\rangle$ ground-state and 0.995(1) (0.996(1)) for the dark $|m_s = -1\rangle \equiv |\downarrow\rangle$ state on Node A (Node B). These values are subsequently used to correct for read-out errors of the electron spins in state tomography measurements.

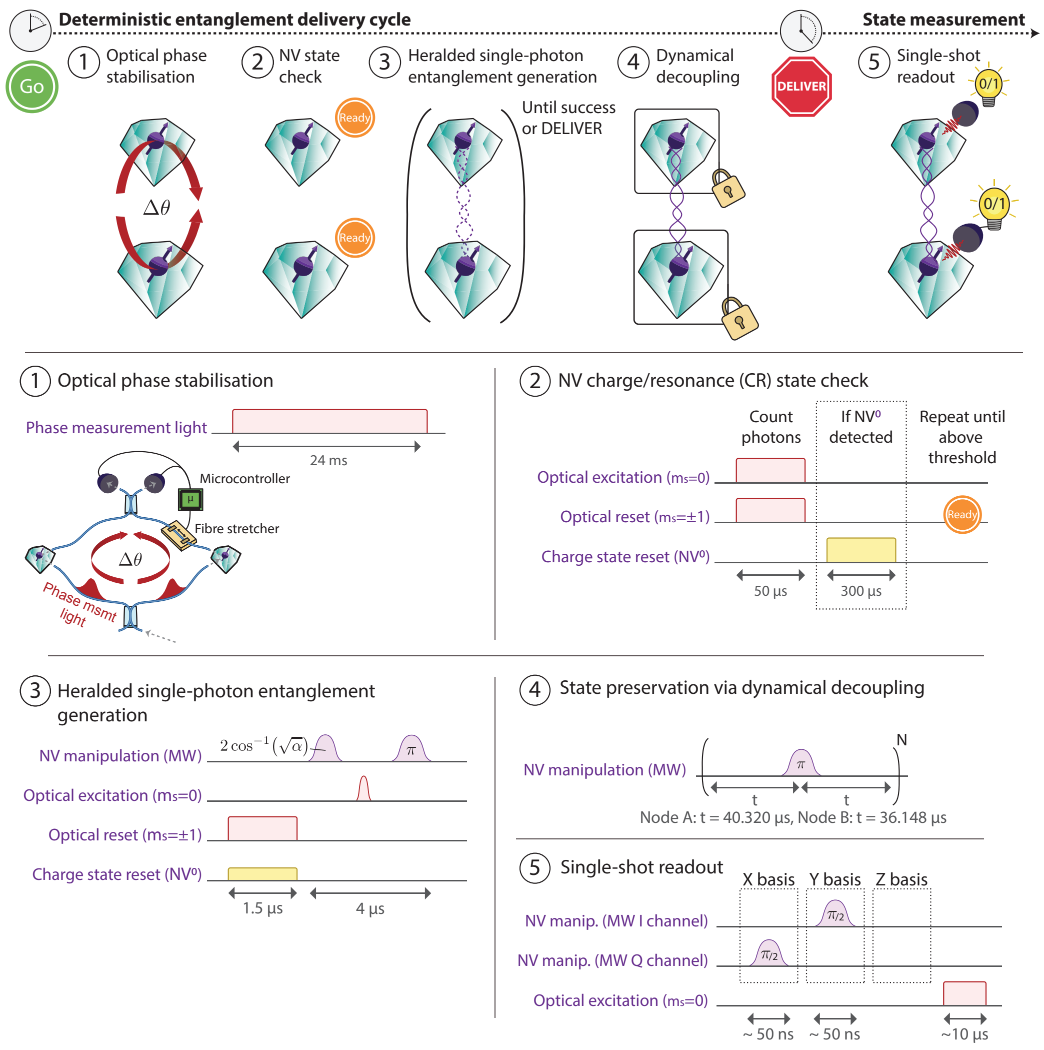


Supplementary Fig. 1. **Deterministic entanglement delivery sequences** Pulse sequences for each step of the deterministic entanglement delivery protocol. These sequences are also employed in the single-photon entanglement generation experiment. ① **Optical phase stabilisation**: Bright light is input to measure and stabilise the interferometer (see Sec. V). Note that the duration is different for the single-photon entanglement experiment. ② **NV state check**: By shining in two lasers that are together resonant with transitions from all of the ground states, the NV will fluoresce regardless of its ground-state occupation. By counting photons emitted by the NV we are able to verify that both NVs are in the desired charge state $NV^-$ and that they are on resonance with the applied lasers. The NV centre is deemed to be on resonance if the number of photons detected during the CR check surpasses a certain threshold [3]. If no photons are detected, the NV is assumed to be in the $NV^0$ state and a resonant laser is applied to reset it to $NV^-$. ③ **Heralded single-photon entanglement generation:** Entanglement generation proceeds by optically repumping the spins to $|\uparrow\rangle$ (including passive charge-state stabilisation, Sec. IV) before a microwave (MW) pulse is used to create the desired bright-state population $\alpha$ at each node. A resonant excitation pulse then generates spin-photon entanglement. A subsequent MW $\pi$ pulse is used to ensure that the NV state is refocused before the next stage should success be heralded. ④ **Dynamical decoupling**: MW pulses are used to implement dynamical decoupling (see Sec. VIII). ⑤ **Single-shot readout**: The NV nodes can be readout in arbitrary bases in a single shot. If required, a MW pulse is applied to rotate the qubit state before a resonant laser is applied. Fluorescence photons from the NV are detected if the NV is in the state $|\uparrow\rangle$ [3].

### B. Independently measured parameters for the experiment

| | Node A | Node B | Description |
|---|---|---|---|
| $T_2$ (ms) | 290(20) | 680(70) | Dephasing time of the electron spin state. |
| $T_1$ (s) | $> 1$ | $> 1$ | Relaxation time of electron spin eigenstates. |
| $p_{\text{det}}$ ($10^{-4}$) | 2.8(1) | 4.2(1) | Probability to detect a ZPL photon after a single excitation. |
| $p_{\text{ionize}}$ | $\leq 10^{-6}$ | $\leq 10^{-6}$ | Probability of passive charge-state control failure per entangling attempt. See Sec. IV. |
| $t$ ($\mu$s) | 40.320 | 36.148 | Optimized inter-pulse delay for state storage. |
| $F_0$ | 0.959(3) | 0.950(3) | Fidelity of the electron read-out for $\|\uparrow\rangle$. |
| $F_{\pm1}$ | 0.995(1) | 0.996(1) | Fidelity of the electron read-out for $\|\downarrow\rangle$. |
| $V$ | 0.90(2) | | Visibility of the two-photon quantum interference. See Sec. VI. |
| $p_{\text{2ph}}$ | 0.04 | | Estimated probability of double excitation during the optical $\pi$-pulse. See Sec. VII. |
| $\nu_{\text{dark}}$ (Hz) | 20 | | Dark count rate per detection channel. |
| $\sigma_{\text{Int}}$ | 14.3(1)° | | Initial uncertainty of the interferometric drift. See Sec. V. |
| $\nu_{\text{Int}}$ ($/s$) | $\sim 20°$ | | Estimated drift rate of the free running interferometer. See Sec. V. |

Supplementary Table I. Independently measured experimental parameters for the performance of the nodes used in our experiment.

### C. Experiment control and communication logic

Supplementary Fig. 2 gives the decision trees and control logic for the ADwin microprocessors (Jaeger ADwin Pro II) that control the experiments. These microcontrollers are responsible for controlling all other experimental hardware and also communicate with each other to synchronise the experiment.

### D. Herald photon detection window

We use a combination of polarization and temporal filtering to separate the excitation pulse from photons emitted by the NV. This necessitates a compromise between collecting as much of the emission light as possible, while ensuring that contamination from the pulse is minimised. In this experiment, we choose a temporal filter window (Supp. Fig. 3) such that the pulse (assumed to have a Gaussian profile) is suppressed to the level of the detector dark counts by the beginning of the window. The end of the window at $\sim 30$ ns after the pulse is chosen so that, for all of the data sets taken, the rate of detected NV photons is greater than ten times the dark count rate at all points within the window. We use a complex programmable logic device (CPLD) to apply this temporal filtering during our experiment and herald the successful generation of an entangled state in real-time.

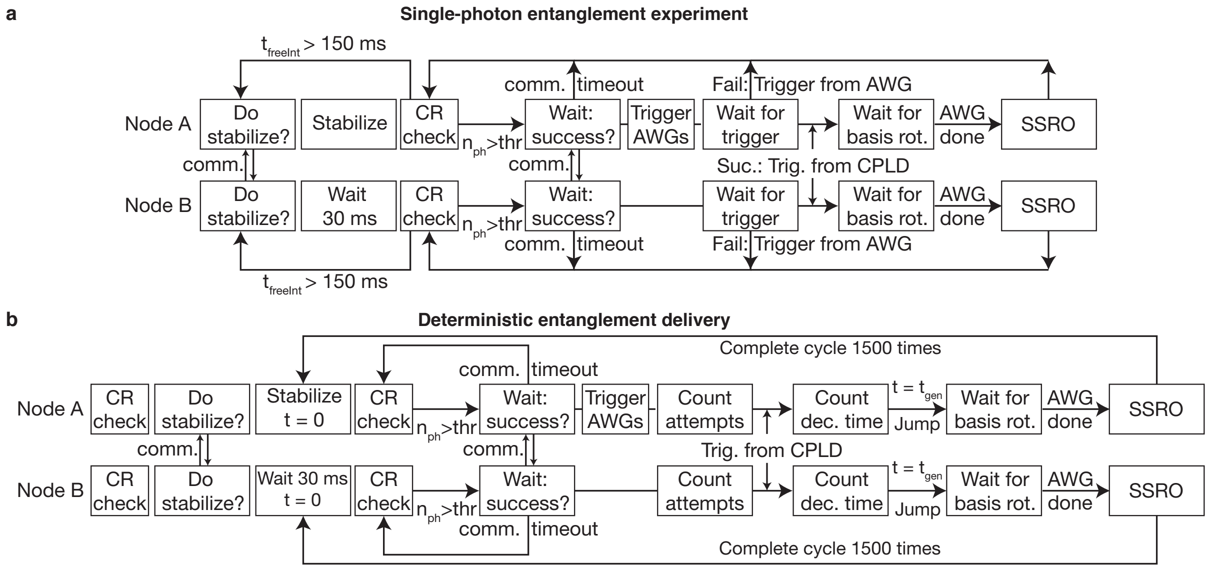


Supplementary Fig. 2. **Flowchart of the experimental sequences.** Shown are the decision trees of the ADwin microprocessors (Jaeger ADwin Pro II) that create the overarching measurement and control loops for network nodes A and B. Both nodes use arbitrary waveform generators for microwave and laser pulse sequencing (AWG, Tektronix AWG5014C). We additionally use a complex programmable logic device (CPLD) to herald the successful generation of an entangled state in real-time (see Sec. II D). **a**. Decision tree when benchmarking the entangled state. **b**. Deterministic entanglement delivery. Here the ADwins keep track of the elapsed time since the end of the phase stabilization ($t = 0$). **CR check**: As explained in Supp. Fig. 1, the NV centre is deemed to be on resonance with the excitation lasers if the number of photons detected during the CR check surpasses a certain threshold $n_{\text{thr}}$. The CR check is repeated until this occurs. **comm. & comm. timeout:** Both ADwins exchange classical communication, such as success of the CR check, via a three-step-handshake. If one ADwin waits longer than 1 ms for a response from its counterpart the communication times out and we return to the previous logical step (see arrow). **Count attempts**: count the number of entangling attempts $N$ until $N = N_{\text{max}}$. **Count dec. time**: track the elapsed time since phase stabilization. If the elapsed time equals the prespecified state-generation time $t_{\text{gen}}$ then trigger the AWG such that the local readout sequences are executed. **Wait for basis rot.**: ADwins wait for a trigger input from the AWG (AWG done) which heralds that the last MW-rotation before optical readout has been completed. **Trigger AWGs**: The ADwin of Node A triggers the AWGs of both nodes to initiate the microwave and entangling sequences. We use a single ADwin as trigger source to avoid timing jitter between both generated sequences. **SSRO**: Optical single-shot read-out. **Success: Trigger from CPLD / Fail: Trigger from AWG**: During entanglement generation, the CPLD communicates successful detection of a photon to the nodes. During the single-photon entanglement benchmarking experiment, the AWG at each node flags failure of the round after 250 entangling attempts. **Do stabilize?**: The ADwins communicate that phase stabilization will be the next step in the experimental sequence. The Node A ADwin then proceeds with the phase stabilization while the ADwin of Node B waits until the phase stabilisation has finished. The deterministic entangling sequence is run a total of 1500 times (500 times per read-out basis) before a new round is called in which starts again with the verification of resonant conditions for both NVs.

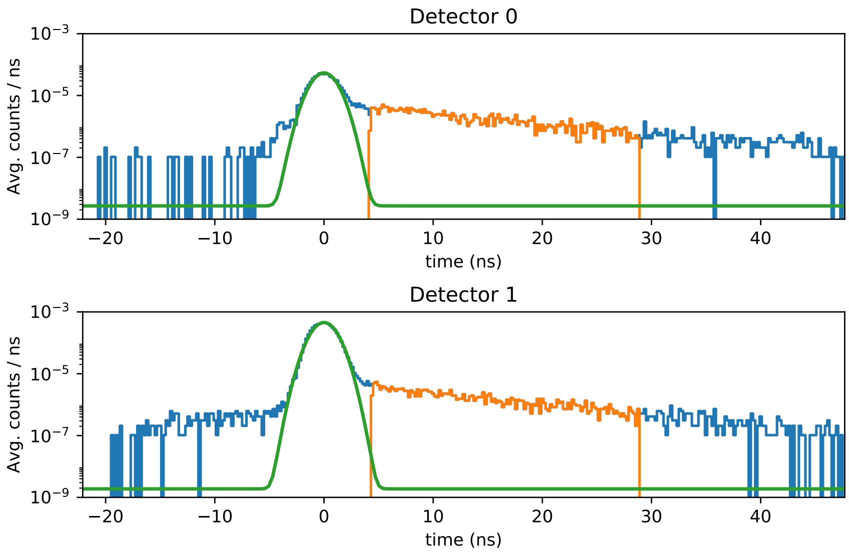


Supplementary Fig. 3. **Temporal filtering of photons.** Histogram of the times at which photons are detected at each single-photon detector (blue) during a deterministic entanglement delivery experiment with bright state population $\alpha = 0.12$. The orange histograms show the photons that were detected within the temporal filter window and therefore were counted as valid entanglement events. The green line shows a gaussian fit to the pulse with a FWHM of 2.26 as measured in Supp. Fig. 7. This is used to estimate the contribution of residual pulse photons within the filter window.

## III. THEORETICAL MODEL OF DETERMINISTIC ENTANGLEMENT DELIVERY

We developed a detailed model to determine the expected performance of the deterministic entanglement delivery experiment, based on the independently measured parameters given in Supplementary Table I.

Once the set-ups are determined to be ready, the core entanglement sequence begins with single-photon entanglement generation. This proceeds by first initialising each node in $|\uparrow\rangle$, followed by a coherent rotation using a microwave pulse to create the state

$$|NV\rangle = \sqrt{\alpha}\,|\uparrow\rangle + \sqrt{1-\alpha}\,|\downarrow\rangle\,. \tag{6}$$

Resonant excitation of the NV nodes excites only the 'bright' $|\uparrow\rangle$ level to an excited state, which rapidly decays radiatively back to the ground state by emitting a single photon. This entangles the state of the NV with the presence $|1\rangle$ or absence $|0\rangle$ of a photon in the emitted optical mode:

$$|NV, \text{optical mode}\rangle = \sqrt{\alpha}\,|\uparrow\rangle\,|1\rangle + \sqrt{1-\alpha}\,|\downarrow\rangle\,|0\rangle\,. \tag{7}$$

The photons emitted by each NV are transmitted to a central station at which a beam-splitter is used to remove their which-path information. Successful detection of a photon at this station indicates that at least one of the NVs is in the bright state $|\uparrow\rangle$ and therefore heralds the creation of a spin-spin entangled state. This entangled state, expressed as $|NV_{\text{Node A}}, NV_{\text{Node B}}\rangle$, is given (in unnormalised form) by

$$\rho_{\text{sc}} = \left|\psi^{\pm}\right\rangle\left\langle\psi^{\pm}\right| + p_{\uparrow\uparrow}\,|\uparrow\uparrow\rangle\langle\uparrow\uparrow| + p_{\downarrow\downarrow}\,|\downarrow\downarrow\rangle\langle\downarrow\downarrow|\,, \tag{8}$$

where

$$\left|\psi^{\pm}\right\rangle\left\langle\psi^{\pm}\right| = \begin{pmatrix} 0 & 0 & 0 & 0 \\ 0 & p_{\uparrow\downarrow} & \pm\sqrt{V\,p_{\uparrow\downarrow}\,p_{\downarrow\uparrow}} & 0 \\ 0 & \pm\sqrt{V\,p_{\uparrow\downarrow}\,p_{\downarrow\uparrow}} & p_{\downarrow\uparrow} & 0 \\ 0 & 0 & 0 & 0 \end{pmatrix}. \tag{9}$$

This state is parametrized by

$$\begin{aligned} p_{\uparrow\uparrow} &= \alpha^2\left((1-p_{\text{dc}})^2(p^A_{\text{det}}(1-p^B_{\text{det}}) + p^B_{\text{det}}(1-p^A_{\text{det}})) \right.\\ &\qquad \left. + 2(1-p_{\text{dc}})\,p_{\text{dc}}(1-p^A_{\text{det}})(1-p^B_{\text{det}})\right) \\ p_{\uparrow\downarrow} &= \alpha\,(1-\alpha)\left((1-p_{\text{dc}})^2\,p^A_{\text{det}} + 2\,p_{\text{dc}}(1-p_{\text{dc}})(1-p^A_{\text{det}})\right) \\ p_{\downarrow\uparrow} &= \alpha\,(1-\alpha)\left((1-p_{\text{dc}})^2\,p^B_{\text{det}} + 2\,p_{\text{dc}}(1-p_{\text{dc}})(1-p^B_{\text{det}})\right) \\ p_{\downarrow\downarrow} &= 2\,(1-\alpha)^2\,p_{\text{dc}}\,(1-p_{\text{dc}}) \end{aligned} \tag{10}$$

where $V$ gives the visibility of two-photon interference, $p_{\text{dc}}$ gives the dark count probability per detector (given by the product of the dark count rate $\nu_{\text{dark}}$ and the 25 ns detection window length), and $p^A_{\text{det}}$ ($p^B_{\text{det}}$) gives the probability of detecting a photon emitted by Node A (B). In the limit of $p_{\text{det}} \ll 1$, for balanced detection probabilities $p_{\text{det}} = p^A_{\text{det}} = p^B_{\text{det}}$ and no other imperfections, this tends to the expression given in the main text: $\rho_{NV,NV} = (1-\alpha)\,|\psi\rangle\langle\psi| + \alpha\,|\uparrow\uparrow\rangle\langle\uparrow\uparrow|$.

We model double excitation (Sec. VII) by applying a Pauli Z transformation to each of the NV states with probability $p_{\text{2ph}}/2$. Phase instability is modelled similarly by applying a

Pauli Z transformation to one of the states with probability $\frac{1}{2}(1 - e^{-\frac{1}{2}((\nu_{\mathrm{Int}} t_p)^2 + \sigma^2_{\mathrm{Int}})})$, where $t_p$ denotes the time elapsed since phase stabilisation.

Finally, we model the impact of dynamical decoupling by assuming that it acts as a depolarising channel for each qubit. We therefore apply single-qubit depolarising errors with a probability determined by the measured dynamical-decoupling coherence times. For decoupling for a total time duration of $t_d$, the total probability of a depolarising error (i.e. the application of a Pauli X, Y or Z transformation with an equal probability) is given by $\frac{3}{4}(1 - e^{-t_d/T_2})$.

## IV. PASSIVE CHARGE-STATE STABILIZATION OF INDIVIDUAL NV CENTRES

The negatively charged NV centre ($NV^-$) can be ionized under optical illumination via a two-photon absorption process [4]. Due to the different level structure of the neutral charge state $NV^0$, the NV will remain dark if such an ionization event occurs during one of our entangling attempts. Ionization thus hampers the performance of our deterministic entangling protocol by diminishing the success rate and delivery of a separable state upon success. Previous experiments with NV centres that worked in the regime of probabilistically generated, yet heralded, remote entanglement overcame NV-ionization by frequent charge-state verification between protocols and actively converting the NV centre back to $NV^-$ by interleaved resonant excitation of the optical transitions of $NV^0$[5].

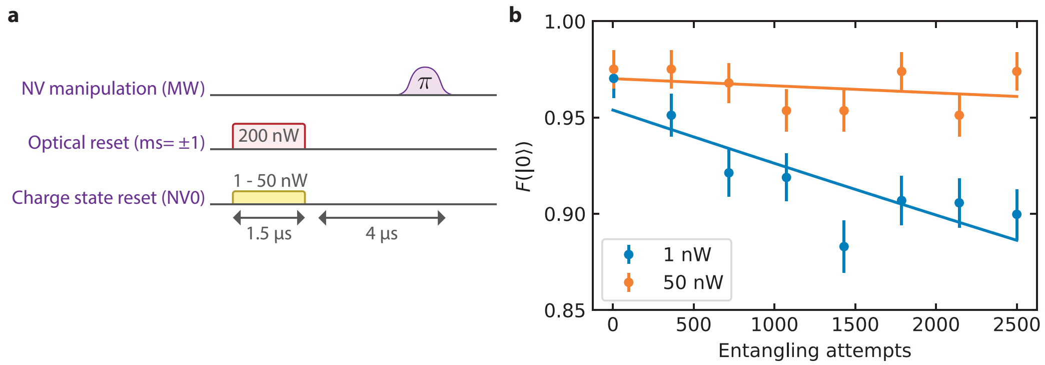


Supplementary Fig. 4. **Verifying passive charge-state stabilization into NV$^-$**. **a**, Elementary sequence to probe the NV ionization rate. **b**, Applying our sequence many times results in a decay of the NV readout fidelity due to ionization. By exploring the ionization rate for different charge-reset powers we find an optimal regime in which the spin initialization of $NV^-$ is not affected by the additional blue-detuned beam and ionization is effectively mitigated over thousands of trials.

Such active stabilization protocols would require additional logical overhead in our scenario where entanglement is generated deterministically. Instead we passively stabilize the charge-state during our entangling sequence by shining in an additional weak laser beam that is resonant with the optical transition of $NV^0$ (Supp. Fig. 4). This provides negligible disturbance to the spin initialization fidelity of $NV^-$ while bringing the NV centre back into $NV^-$ if it was converted to $NV^0$. We additionally identify that the optical reset beam (duration $1.5\,\mu$s) is the main cause of ionization in our system and carefully balance the

power of both beams such that the spin state is still well initialized and that ionization is a negligible process for our deterministic entangling protocol (up to 15000 entangling attempts). Note that reducing the applied power further by elongating the spin reset duration would decrease the entanglement rate and limit our quantum link efficiency.

Figure 4 depicts the basic element that, in repetition, forms our sequence to probe the ionization rate. We use simultaneous charge and spin reset beams followed by a single microwave $\pi$ rotation that brings the NV into $|1\rangle$ and thus guarantees optical excitation during the next round. The NV is then readout after a final optical reinitialisation into the bright state $|0\rangle$. By increasing the number of sequence repetitions, we observe a decay of the final readout fidelity that is associated with the ionization rate. By increasing the optical intensity of the charge-state reset beam we obtain a negligible decay as a function of sequence repetitions, therefore allowing us to overcome ionization in our deterministic entangling protocol. Note that the illumination strength of the charge-reset beam is weak enough to avoid inducing noticeable spectral diffusion of the NV emission as our measured entangled states are consistent with a high degree of indistinguishability for both NV emission profiles (see Secs. VI).

## V. OPTICAL PHASE STABILISATION

The single-photon entanglement experiment requires that optical phase of an effective interferometer between the two nodes is known, as shown in Fig. 2 of the main text. The optical phase difference between the paths of this interferometer must be known in order to ensure that entangled states are available for further use. This is achieved by interleaving periods of optical-phase stabilisation with our entanglement generation.

For phase stabilisation we input bright laser light at the same frequency but orthogonally polarised to the light used for excitation of the NVs. The orthogonal polarisation is chosen because we use a crossed-polariser to filter out the excitation light from the NV emission. Using orthogonally polarised light for phase stabilisation therefore allows us to collect more light reflected from the diamond substrate. Before doing this, we verified that there is no measurable difference in the relative phase of the two polarisations within our interferometer.

Measurements of the phase drift (Supp. Fig. 5a) show a slow drift on second time scales, but several strong resonances at hundreds of hertz (Supp. Fig. 5b). These resonances are thought to be from mechanical elements in the path of the beam, including the microscope objective mount. As we were unable to completely suppress these resonances in the current set-ups, we need to measure the phase over a complete oscillation to estimate the mean phase reliably. The phase must therefore be measured for approximately 10 ms.

We calculate an estimate of the phase from the counts detected at the heralding single-photon detectors. This estimate is used to adjust the phase back to our desired value using a homebuilt piezoelectric fibre stretcher and a proportional-integral-derivative (PID) routine within our Adwin micro-controller. We find that it takes between 2-3 PID cycles to optimally stabilise the phase. We stabilise the phase for 3 cycles during the single-photon entanglement experiment and for 2 cycles during the deterministic entanglement experiment. This difference is because phase stabilisation occurs during every cycle of the deterministic entanglement delivery experiment ( 100 ms), while it only occurs every 180 ms during the single-photon entanglement experiment and therefore the phase drifts slightly less after one experimental cycle.

We achieve an average steady-state phase stability of $14.3(1)^\circ$, as measured by calibration

routines spaced throughout the measurement of our data set (Supp. Fig. 5c,d). This stability is limited by the previously identified mechanical oscillations of the optical elements in our experimental set-up. The standard deviation of the phase averaged over a 10 ms period during active stabilisation is 4.8(1)°.

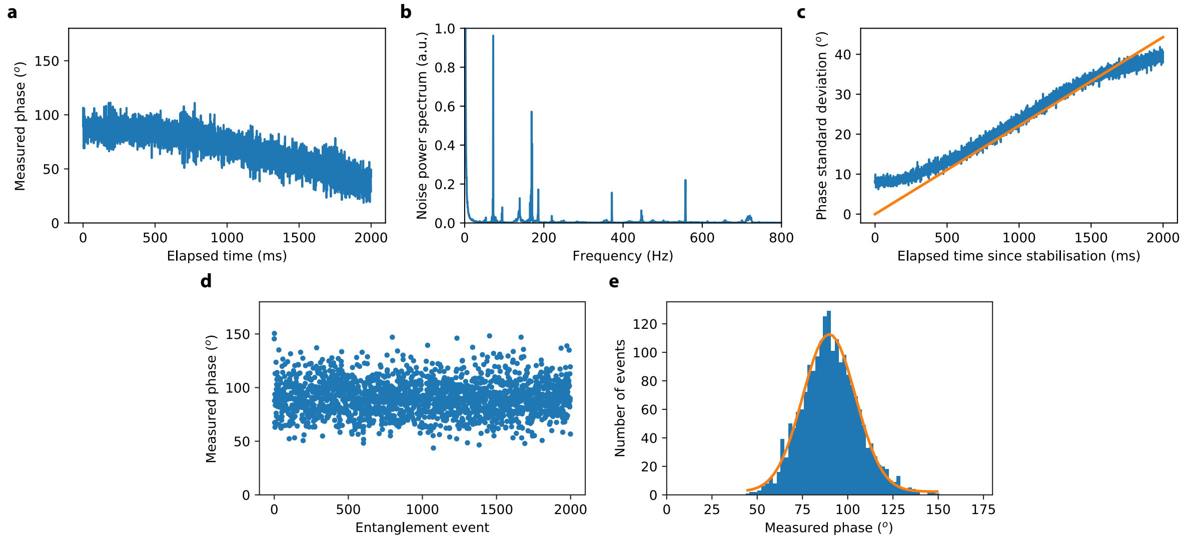


Supplementary Fig. 5. **Optical phase stabilisation.** Single-photon entanglement requires that optical phase of an effective interferometer between the two nodes is known. **a**, A typical trace of the interferometer optical phase as it is passively tracked for two seconds. **b**, Power spectrum of the optical phase signal showing peaks thought to be due to mechanical resonances of components in the setup. **c**, Active phase stabilisation is used to correct for phase drifts. Here the phase is stabilised and then the interferometer is allowed to passively drift for two seconds. Plotted is the standard deviation of the phase as a function of elapsed time for a data set of 100 of these measurements. The orange line shows a linear fit, used to estimate the rate of phase drift $\nu_{\text{Int}} \sim 20°/s$. **d**, Here the phase is repeatedly actively stabilised every 180 ms. Entanglement generation occurs during the periods in between stabilisation. The interferometer phase is measured directly after each successful heralded entanglement event. **e**, Histogram of the measured post-entanglement optical phases. Also plotted in orange is a Gaussian fit with a standard deviation fixed to the average measured standard deviation for all entanglement data taken, $\sigma_{\text{Int}} = 14.3(1)°$.

We note that optical phase stabilisation is also likely to be feasible for long-distance network links. Using long-wavelength off-resonant light for phase measurements would allow for continuous stabilisation during entanglement attempts with negligible impact upon the NV state. An experimental study [6] has shown that two network nodes separated by 36 km over a commercial fibre network would still allow for interference visibilities of 99%. For longer distances, it would also be possible to passively track the phase at the time of entanglement delivery and feed this information back to the nodes in which the state is stored, requiring only a coherence time longer than the communication time.

## VI. TWO-PHOTON QUANTUM INTERFERENCE

The quality of photon-mediated heralded entanglement between two emitters hinges on the indistinguishability of their emitted photons. We probe this indistinguishability by interfering emitted single photons on a beam splitter and measuring the number of events in which single-photon detectors connected to the output ports of the beamsplitter both detect a photon. For completely indistinguishable single photons, Hong-Ou-Mandel interference ensures that both photons always exit from the same port of the beamsplitter, and therefore no coincident events should be detected.

Our TPQI experiment proceeds by exciting each emitter with a series of well separated optical excitation pulses (separated by $1\,\mu$s). We collect statistics on coincidence events in which one detector registers a photon after one excitation pulse, and then the other detector registers a photon after a later excitation pulse. For an infinite pulse train, the number of coincidence events detected for each number of pulses between the detection events should be constant. However, for a finite pulse train, there are some pulses for a given pulse separation for which there is no partner excitation pulse and therefore no coincident events will be detected. This leads to a linearly decreasing number of coincidence events as a function of pulse difference (Supp. Fig. 6a).

We use a linear fit to the coincidence events to infer the number of coincidences that would be detected from the same pulse (pulse difference of zero), if fully distinguishable single photons were input (Supp. Fig. 6b). Because these are nonetheless single photons, a counting argument shows that, for balanced emission probabilities from each emitter, this expected number of events is given by half of the value of the linear fit at zero pulse difference.

The ratio $r$ between the measured number of coincident events within the same pulse and the expected number of events for fully distinguishable photons is related to the single-photon wave function overlap $V = |\langle\psi_a|\,\psi_b\rangle|^2$ by $V = (1-r)$ (again for balanced emission probabilities from each emitter). Incorporating the effect of the known imbalance in emission probabilities in our experiment, we find $V = 0.90(2)$.

## VII. DEPHASING OF ENTANGLED STATES DUE TO DOUBLE EXCITATION

An optical rabi pulse is used to excite the NV nodes to a higher lying level via a spin-conserving transition. The NV subsequently decays back down to its original level through spontaneous emission, thereby entangling the spin state of the NV and the emitted optical mode. For optical rabi pulses of finite duration, there is a chance that the NV will spontaneously emit a photon during the optical pulse and be re-excited before the end of the pulse. the first emitted photon will be lost to the environment, as it is impossible to distinguish from the excitation light. However, if the subsequent emitted photon is detected in this double excitation process, this will falsely herald entanglement. We measured the width of our optical pulse (Supp. Fig. 7) and used a quantum-jump based simulation to calculate the corresponding double-excitation probability. Given that the NV emitted a photon within the detection window, the probability that double excitation occurred is $p_{\mathrm{2ph}} = 0.04$.

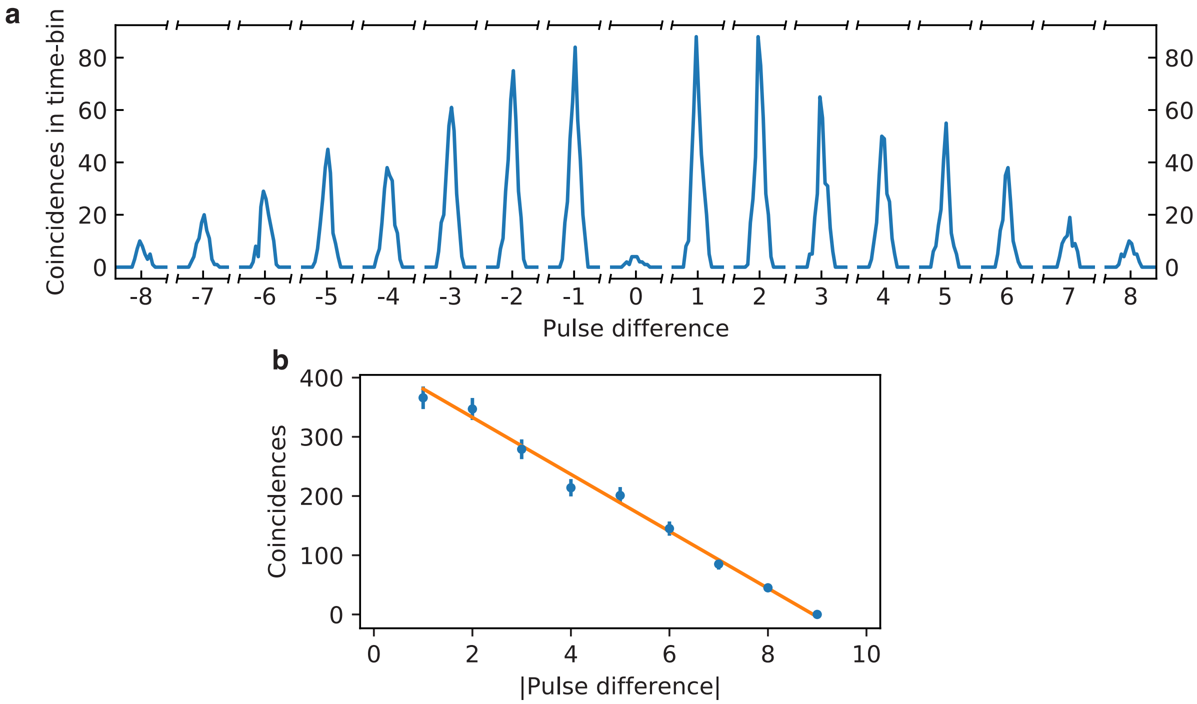


Supplementary Fig. 6. **Two-photon quantum interference. a**. Histogram for coincident events measured by two single-photon detectors in a two-photon quantum interference experiment, measured by cross-referencing photon detection events from a pulse train of 10 optical $\pi$-pulses that excite both emitters. Hong-Ou-Mandel interference of simultaneously coinciding photons ideally results in vanishing coincidence events within a single excitation round. The time difference between individual excitation rounds is $1\,\mu$s. Histograms of coincidence counts are shown with a bin-size of 5 ns. **b**. Total number of coincidences as a function of the number of pulses separating the two detection events. We extrapolate the measured coincidences to infer the expected coincidences for distinguishable photons at zero pulse difference by fitting a linear regression (orange). Using this to normalise the 22 observed coincidences for zero pulse difference allows us to estimate the TPQI visibility $V = 0.90(2)$.

## VIII. STATE STORAGE VIA DYNAMICAL DECOUPLING

The coherence time of NV centres is limited by interactions with other magnetic impurities. In our samples the dominant source of magnetic field noise is the surrounding bath of slowly fluctuating $^{13}$C nuclear spins (natural abundance of 1.1 %) resulting in typical coherence times of $5\,\mu$s. We use dynamical decoupling XY8 sequences of the form $(t - \pi_X - 2t - \pi_Y - 2t - \pi_X - 2t - \pi_Y - 2t - \pi_Y - 2t - \pi_X - 2t - \pi_Y - 2t - \pi_X - t)^{N/8}$ to elongate the coherence times of both NV centres (see Fig. 3 main text), with microwave inversion pulses $\pi$, the waiting time $t$ and the number of pulses $N$ (see also Supp. Fig. 1.4). A given decoupling duration is obtained by arbitrary combinations of $t$ and $N$. We find the optimal combination for a targeted protection duration of $\sim 100$ ms by varying $t$ for a fixed $N = 1024$. We specifically choose $N = 1024$ as the introduced infidelity from inversion pulse errors is still moderate for both nodes.

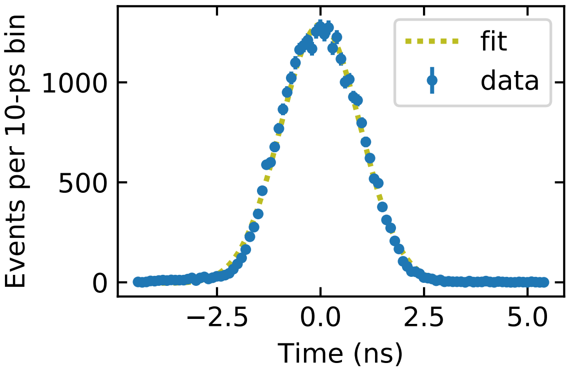


Supplementary Fig. 7. **Width of the optical $\pi$-pulse**. FWHM = 2.26 ns, necessary to compute the dual-excitation probability for a radiative lifetime of 12 ns

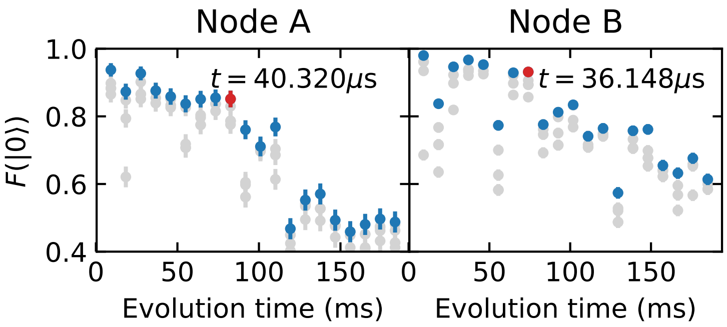


Supplementary Fig. 8. **Determining the optimal inter-pulse delay for state storage and 1024 inversion pulses.** We initialize a superposition state on the NV electron spin, preserve it via dynamical decoupling and finally perform optical readout after another $\pi/2$ pulse. We probe the coherence of the NV by varying the inter-pulse delay $t$ in steps of the Larmor period $1/\nu_L \approx 2.25\,\mu$s and additionally shifting the delay in steps of 4 ns for a total of five data points per Larmor period (grey data). For each multiple of the Larmor period we pick the best, i.e. most preserving, inter-pulse delay (blue data). We determine the optimal delay $t$ by selecting an inter-pulse delay that provides sufficient state preservation, i.e. $\sim$ 100 ms, for a moderate amount of pulses (red data point and text inset in both panels). Left: Node A. Right: Node B. Error bars are 1 s.d.

Figure 8 shows the results of our decoupling optimization procedure. We prepare the NV in a balanced superposition and choose waiting times that are integer multiples of the inverse $^{13}$C-nuclear-spin Larmor frequency $\nu_L$ to avoid coupling with the nuclear spin bath (Node A: $\nu_L$ = 443.342 kHz; Node B: $\nu_L$ = 442.442 kHz). Following the techniques of Abobeih et al. [7], we further avoid coupling to other magnetic noise sources that result in loss of NV coherence by picking five waiting times with a total variation of 16 ns for each multiple of the inverse Larmor frequency. The data (grey) are then sorted for the waiting time with the best state preservation quality (blue) at each multiple, giving the minimal NV coherence decay for this number of inversion pulses. We then proceed to pick the waiting time that guarantees

a low number of inversion pulses while still providing high-quality state protection (red).

---

[1] Hensen, B. *et al.* Loophole-free Bell inequality violation using electron spins separated by 1.3 kilometres. *Nature* **526**, 682–686 (2015).

[2] Kalb, N. *et al.* Entanglement distillation between solid-state quantum network nodes. *Science* **356**, 928–932 (2017).

[3] Robledo, L. *et al.* High-fidelity projective read-out of a solid-state spin quantum register. *Nature* **477**, 574–578 (2011).

[4] Aslam, N., Waldherr, G., Neumann, P., Jelezko, F. & Wrachtrup, J. Photo-induced ionization dynamics of the nitrogen vacancy defect in diamond investigated by single-shot charge state detection. *New J. Phys.* **15**, 013064 (2013).

[5] Pfaff, W. *et al.* Unconditional quantum teleportation between distant solid-state quantum bits. *Science* **345**, 532–535 (2014).

[6] Minář, J., de Riedmatten, H., Simon, C., Zbinden, H. & Gisin, N. Phase-noise measurements in long-fiber interferometers for quantum-repeater applications. *Phys. Rev. A* **77**, 052325 (2008).

[7] Abobeih, M. & et. al. Manuscript in preparation .
